# Supplementary material for: Detection of Doctored Speech: Towards an End-to-End Parametric Learn-able Filter Approach
Source: arXiv:2206.13066 source file (2022-06-27)
Supplement: Supplementary file 2 [file AppendixTemplate.tex]

% Appendix Template

\chapter{Appendix Title Here} % Main appendix title

\label{AppendixX} % Change X to a consecutive letter; for referencing this appendix elsewhere, use \ref{AppendixX}

Write your Appendix content here.
